# Supplementary material for: Large-Scale Analysis of Online Questions Related to Opioid Use Disorder on Reddit
Source: arXiv:2504.08044 source file (2025-04-10)
Supplement: Supplementary file 1 [file appendix.tex]

\documentclass[../main.tex]{subfiles}

\setcounter{page}{1}

%\counterwithin{figure}{section}

\setcounter{table}{0}

\setcounter{figure}{0}

\begin{document}

\maketitle

\end{document}
